# Supplementary material for: AnimatableDreamer: Text-Guided Non-rigid 3D Model Generation and Reconstruction with Canonical Score Distillation
Source: arXiv:2312.03795 source file (2024-03-28)
Supplement: Supplementary file 1 [file X_suppl.tex]

\clearpage
\appendix
% \onecolumn
\setcounter{page}{1}
\setcounter{proposition}{0}
\setcounter{section}{0}

% \clearpage
% \setcounter{page}{1}
% \maketitlesupplementary
\section{Project Website}
\textbf{For more detailed and intractable results, please visit our Project Website at} \url{https://AnimatableDreamer.github.io/}. 
\section{Additional Ablation Results of Generation}
As depicted in \Cref{fig:sup_abl}, an ablation study was conducted to evaluate the proposed techniques. Specifically, the inclusion of $\mathcal{L}_{skel}$ enhances the coherence between motion and the generated model, ensuring a tighter bond. The model is prone to collapse in the absence of $\mathcal{L}_{\text{skel}}$. Concurrently, $\mathcal{L}_{bone}$ plays a critical role in aligning the generated surface meticulously with the underlying skeletal structure.

\begin{figure*}[!h]
  \centering
  % \fbox{\rule{0pt}{2in} \rule{0.9\linewidth}{0pt}}
   \includegraphics[width=0.7\linewidth]{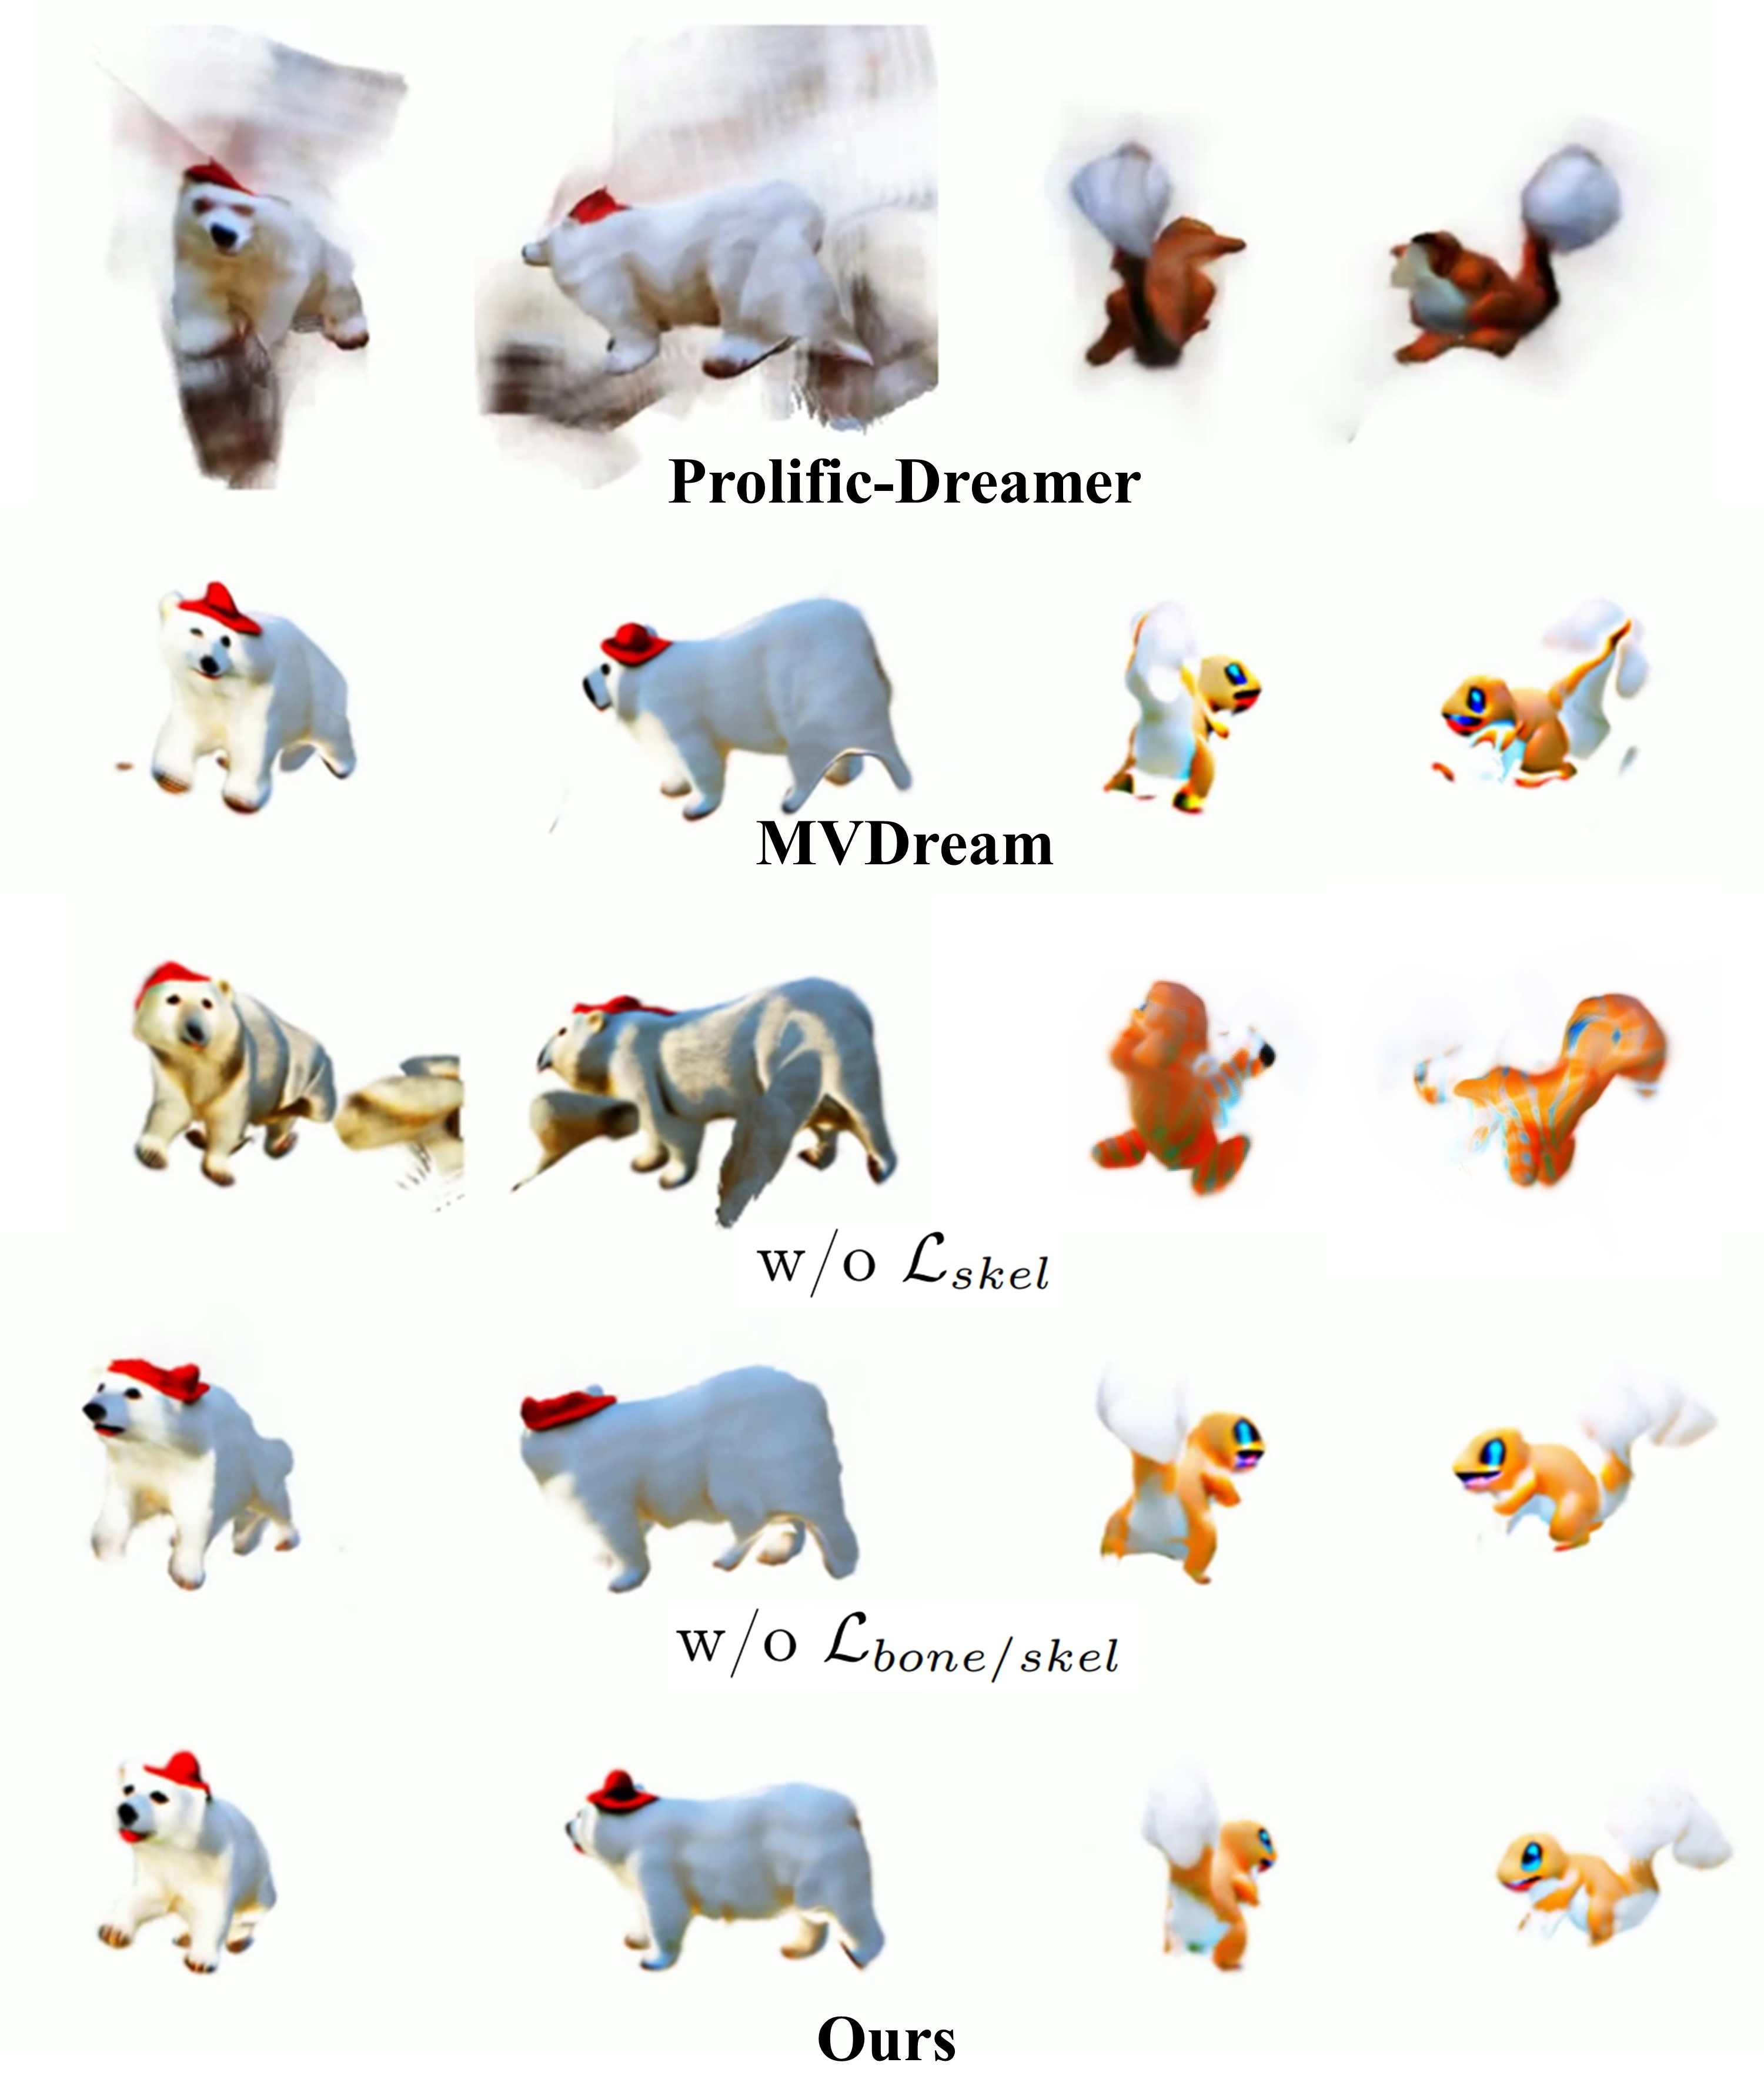}
   \caption{\textbf{Comparison and Ablation study.} The model is prone to collapse in the absence of $\mathcal{L}_{\text{skel}}$. Concurrently, $\mathcal{L}_{\text{bone}}$ plays an indispensable role in precisely aligning the generated surface with the underlying skeletal structure. ProlificDreamer fails to generate meaningful results because of the lack of multi-view information. MVDream generates relatively reasonable result, but degrades after warping.}
   \label{fig:sup_abl}
\end{figure*}
We present visualizations of the skeletal structures in the collapsed case above without $\mathcal{L}_{\text{skel}}$, attributing the collapse to the divergence in bone transformations. To substantiate the efficacy of $\mathcal{L}_{\text{skel}}$, a comparative visualization with $\mathcal{L}_{\text{skel}}$ applied is provided, as shown in \Cref{fig:sup_vis_skel}.
\begin{figure*}[!h]
  \centering
  % \fbox{\rule{0pt}{2in} \rule{0.9\linewidth}{0pt}}
   \includegraphics[width=0.8\linewidth]{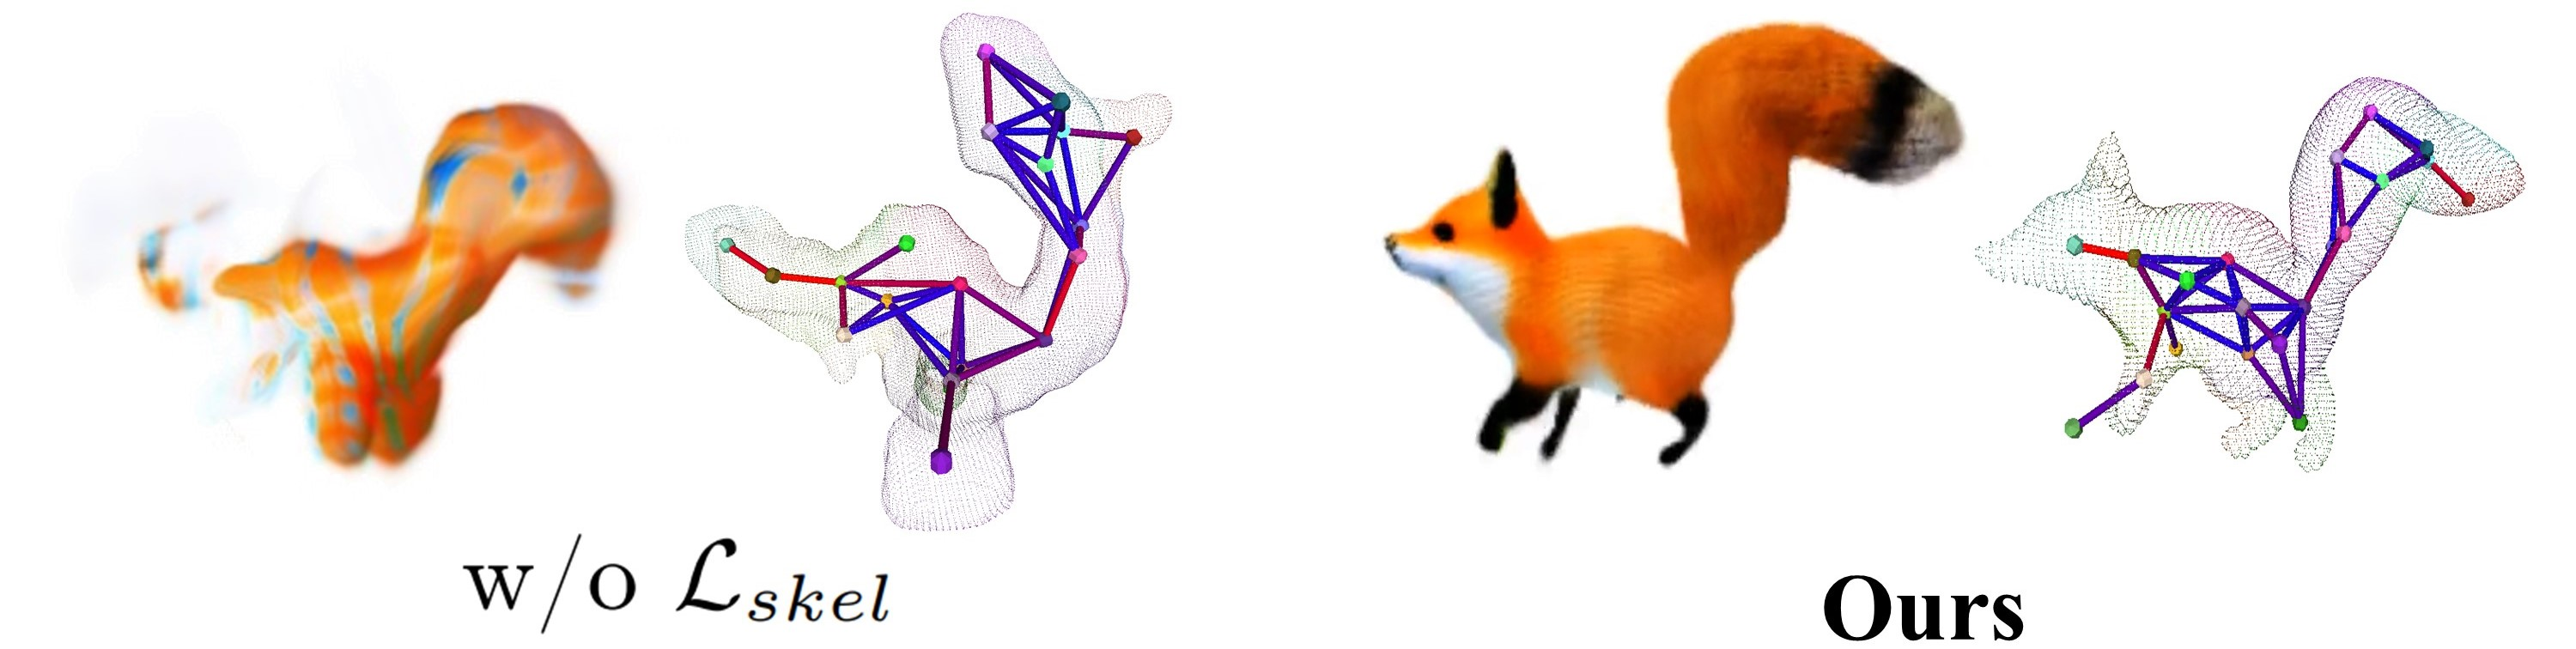}
   \caption{\textbf{Bone transformations diverge without skeleton restriction.} The bones go into implausible positions without skeleton restriction.}
   \label{fig:sup_vis_skel}
\end{figure*}

\section{Additional Generation Results}
We present additional results of AnimatableDreamer for non-rigid generation in \Cref{fig:sup_gen}. AnimatableDreamer exhibits robust generalization performance across various types of non-rigid objects. In addition to the generation of texture, the geometry is also produced.
\begin{figure*}[!h]
  \centering
  % \fbox{\rule{0pt}{2in} \rule{0.9\linewidth}{0pt}}
   \includegraphics[width=0.95\linewidth]{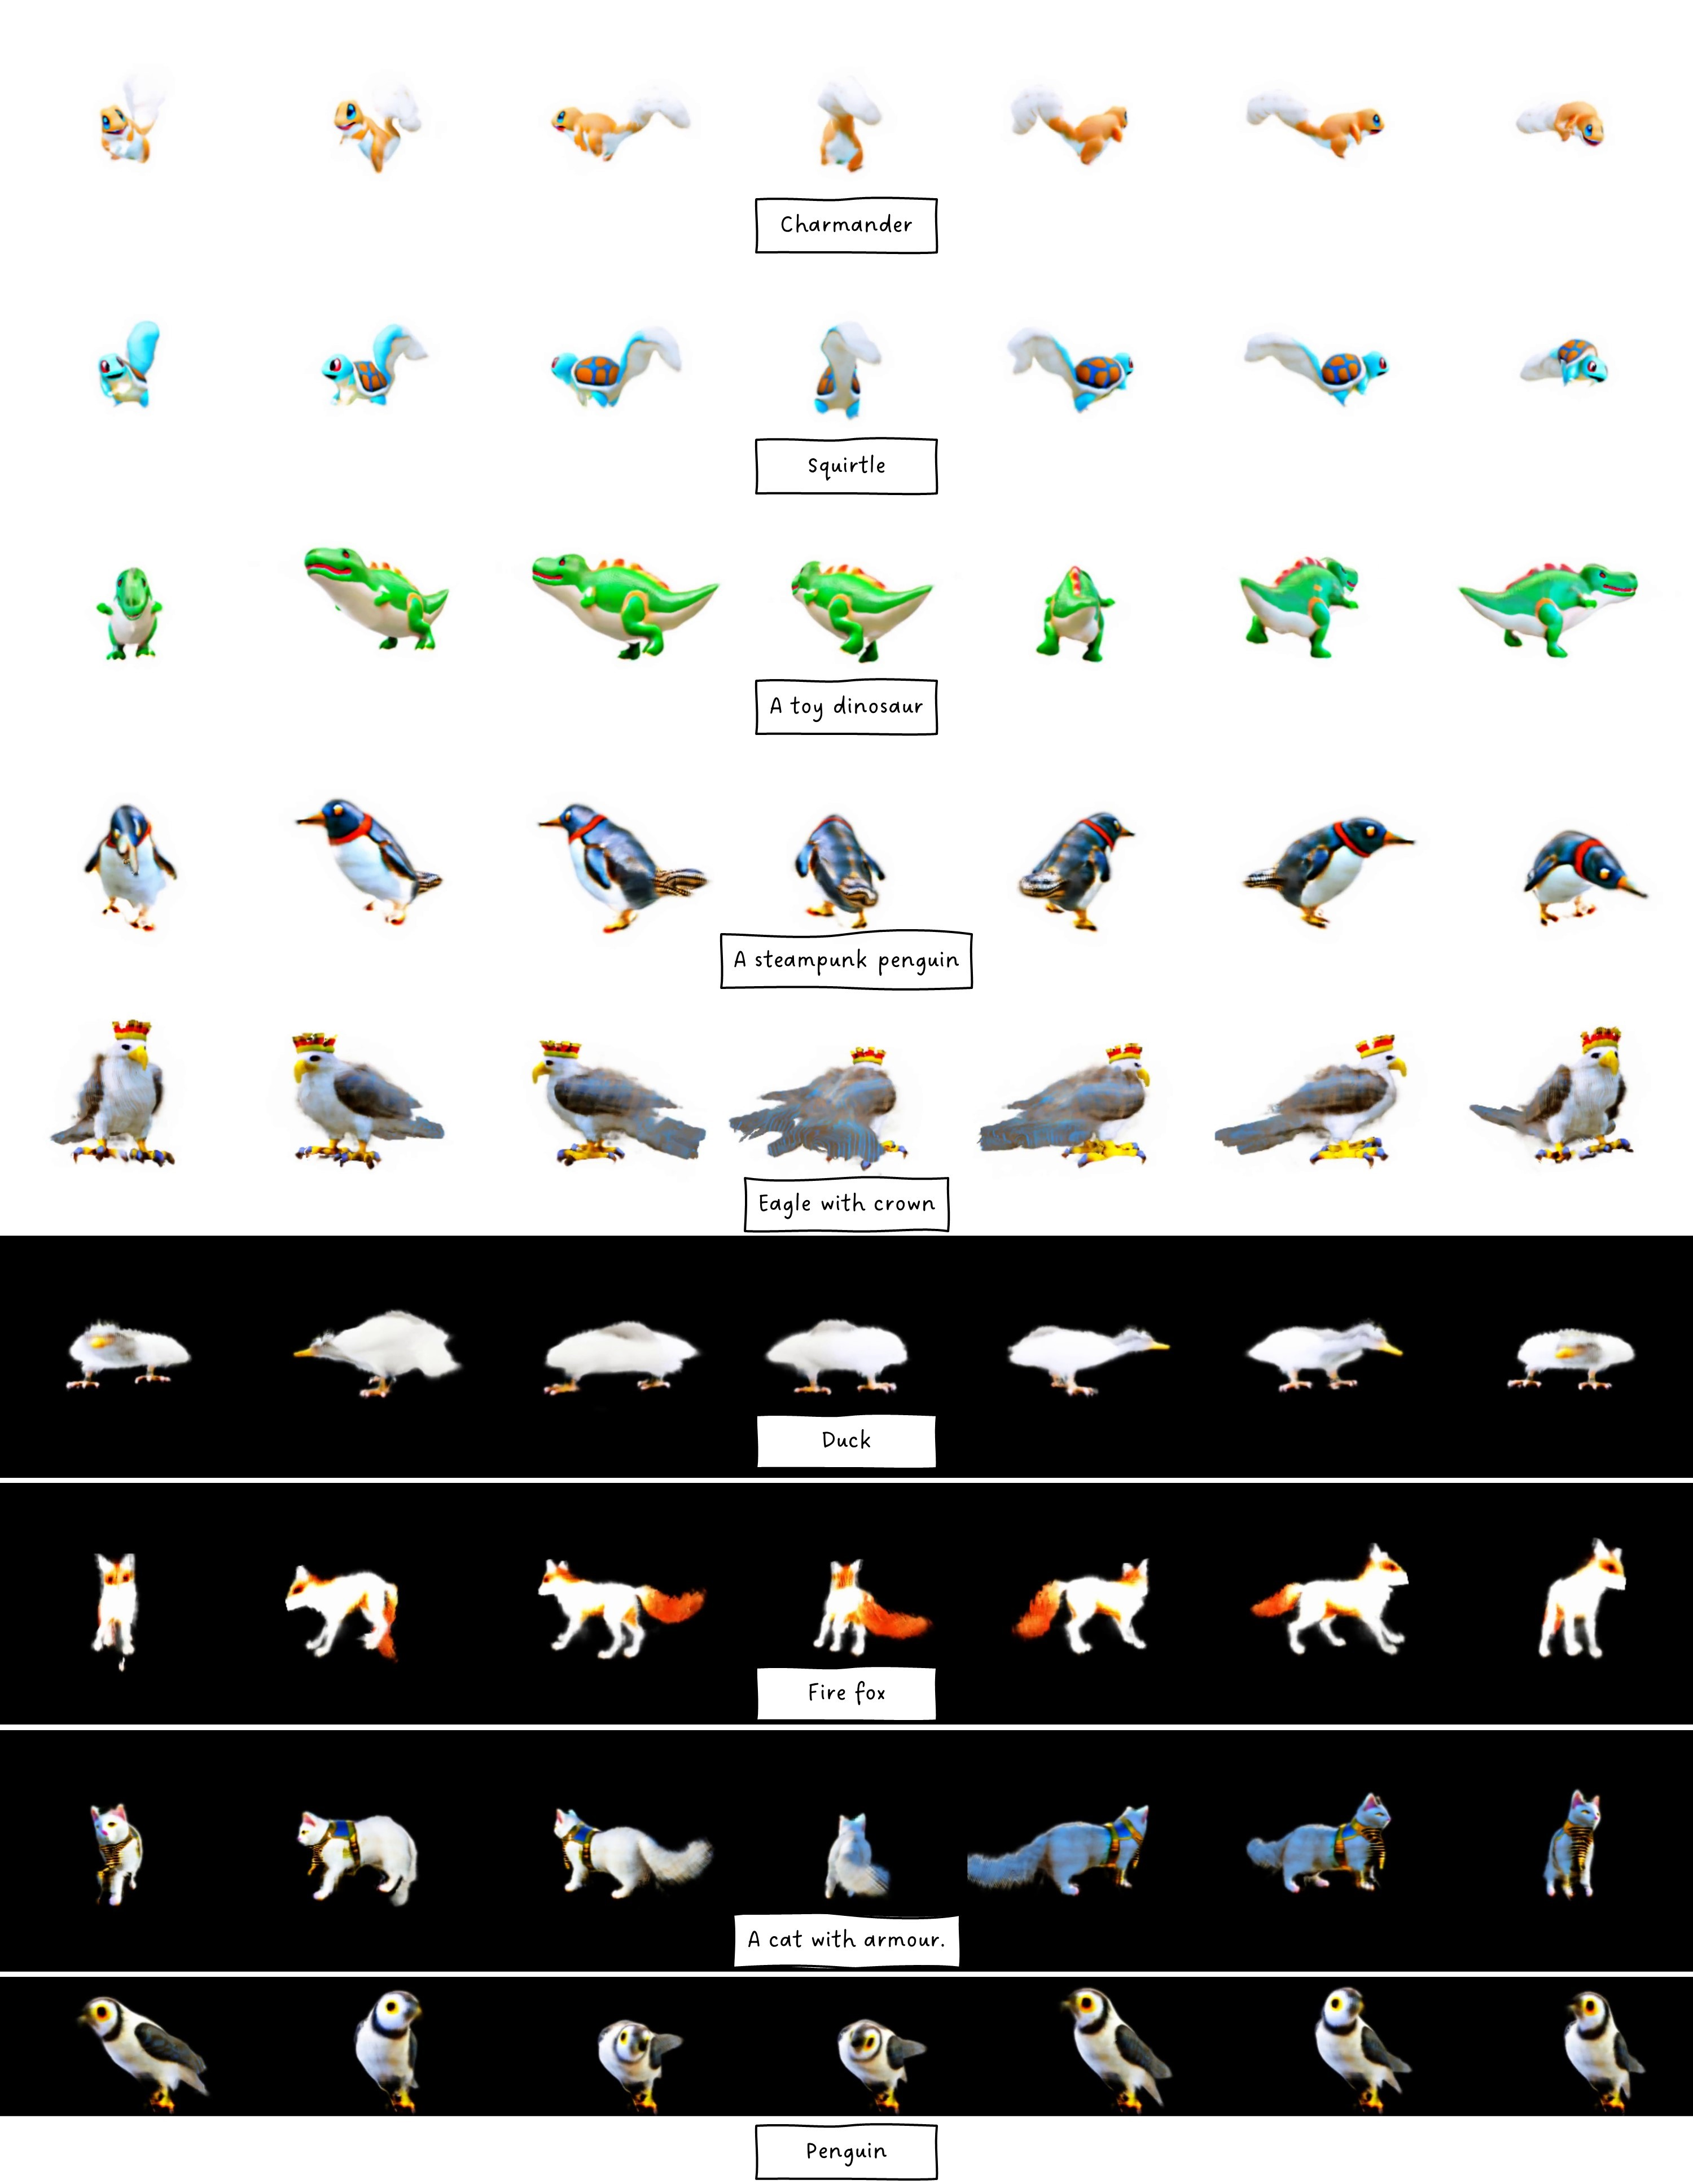}
   \caption{\textbf{Results of high-quality animatable models from AnimatableDreamer.} In addition to the generation of texture, geometry is also produced. Here we set the background to black in some cases for better generation.}
   \label{fig:sup_gen}
\end{figure*}
\section{Additional Reconstruction Results}
We present additional results of AnimatableDreamer for non-rigid reconstruction in \Cref{fig:sup_recon}. In contrast to existing methods, our framework effectively completes the unobserved regions on the 3D model, leveraging the inductive priors and instance information provided by the multi-view diffusion model. We also visualize the extract skeletons with animations in \Cref{fig:sup_anim}.
% \section{The derivation of CSD} CSD is in a form combining gradient from the warping field and canonical field. 

\begin{figure*}[!h]
  \centering
  % \fbox{\rule{0pt}{2in} \rule{0.9\linewidth}{0pt}}
   \includegraphics[width=0.95\linewidth]{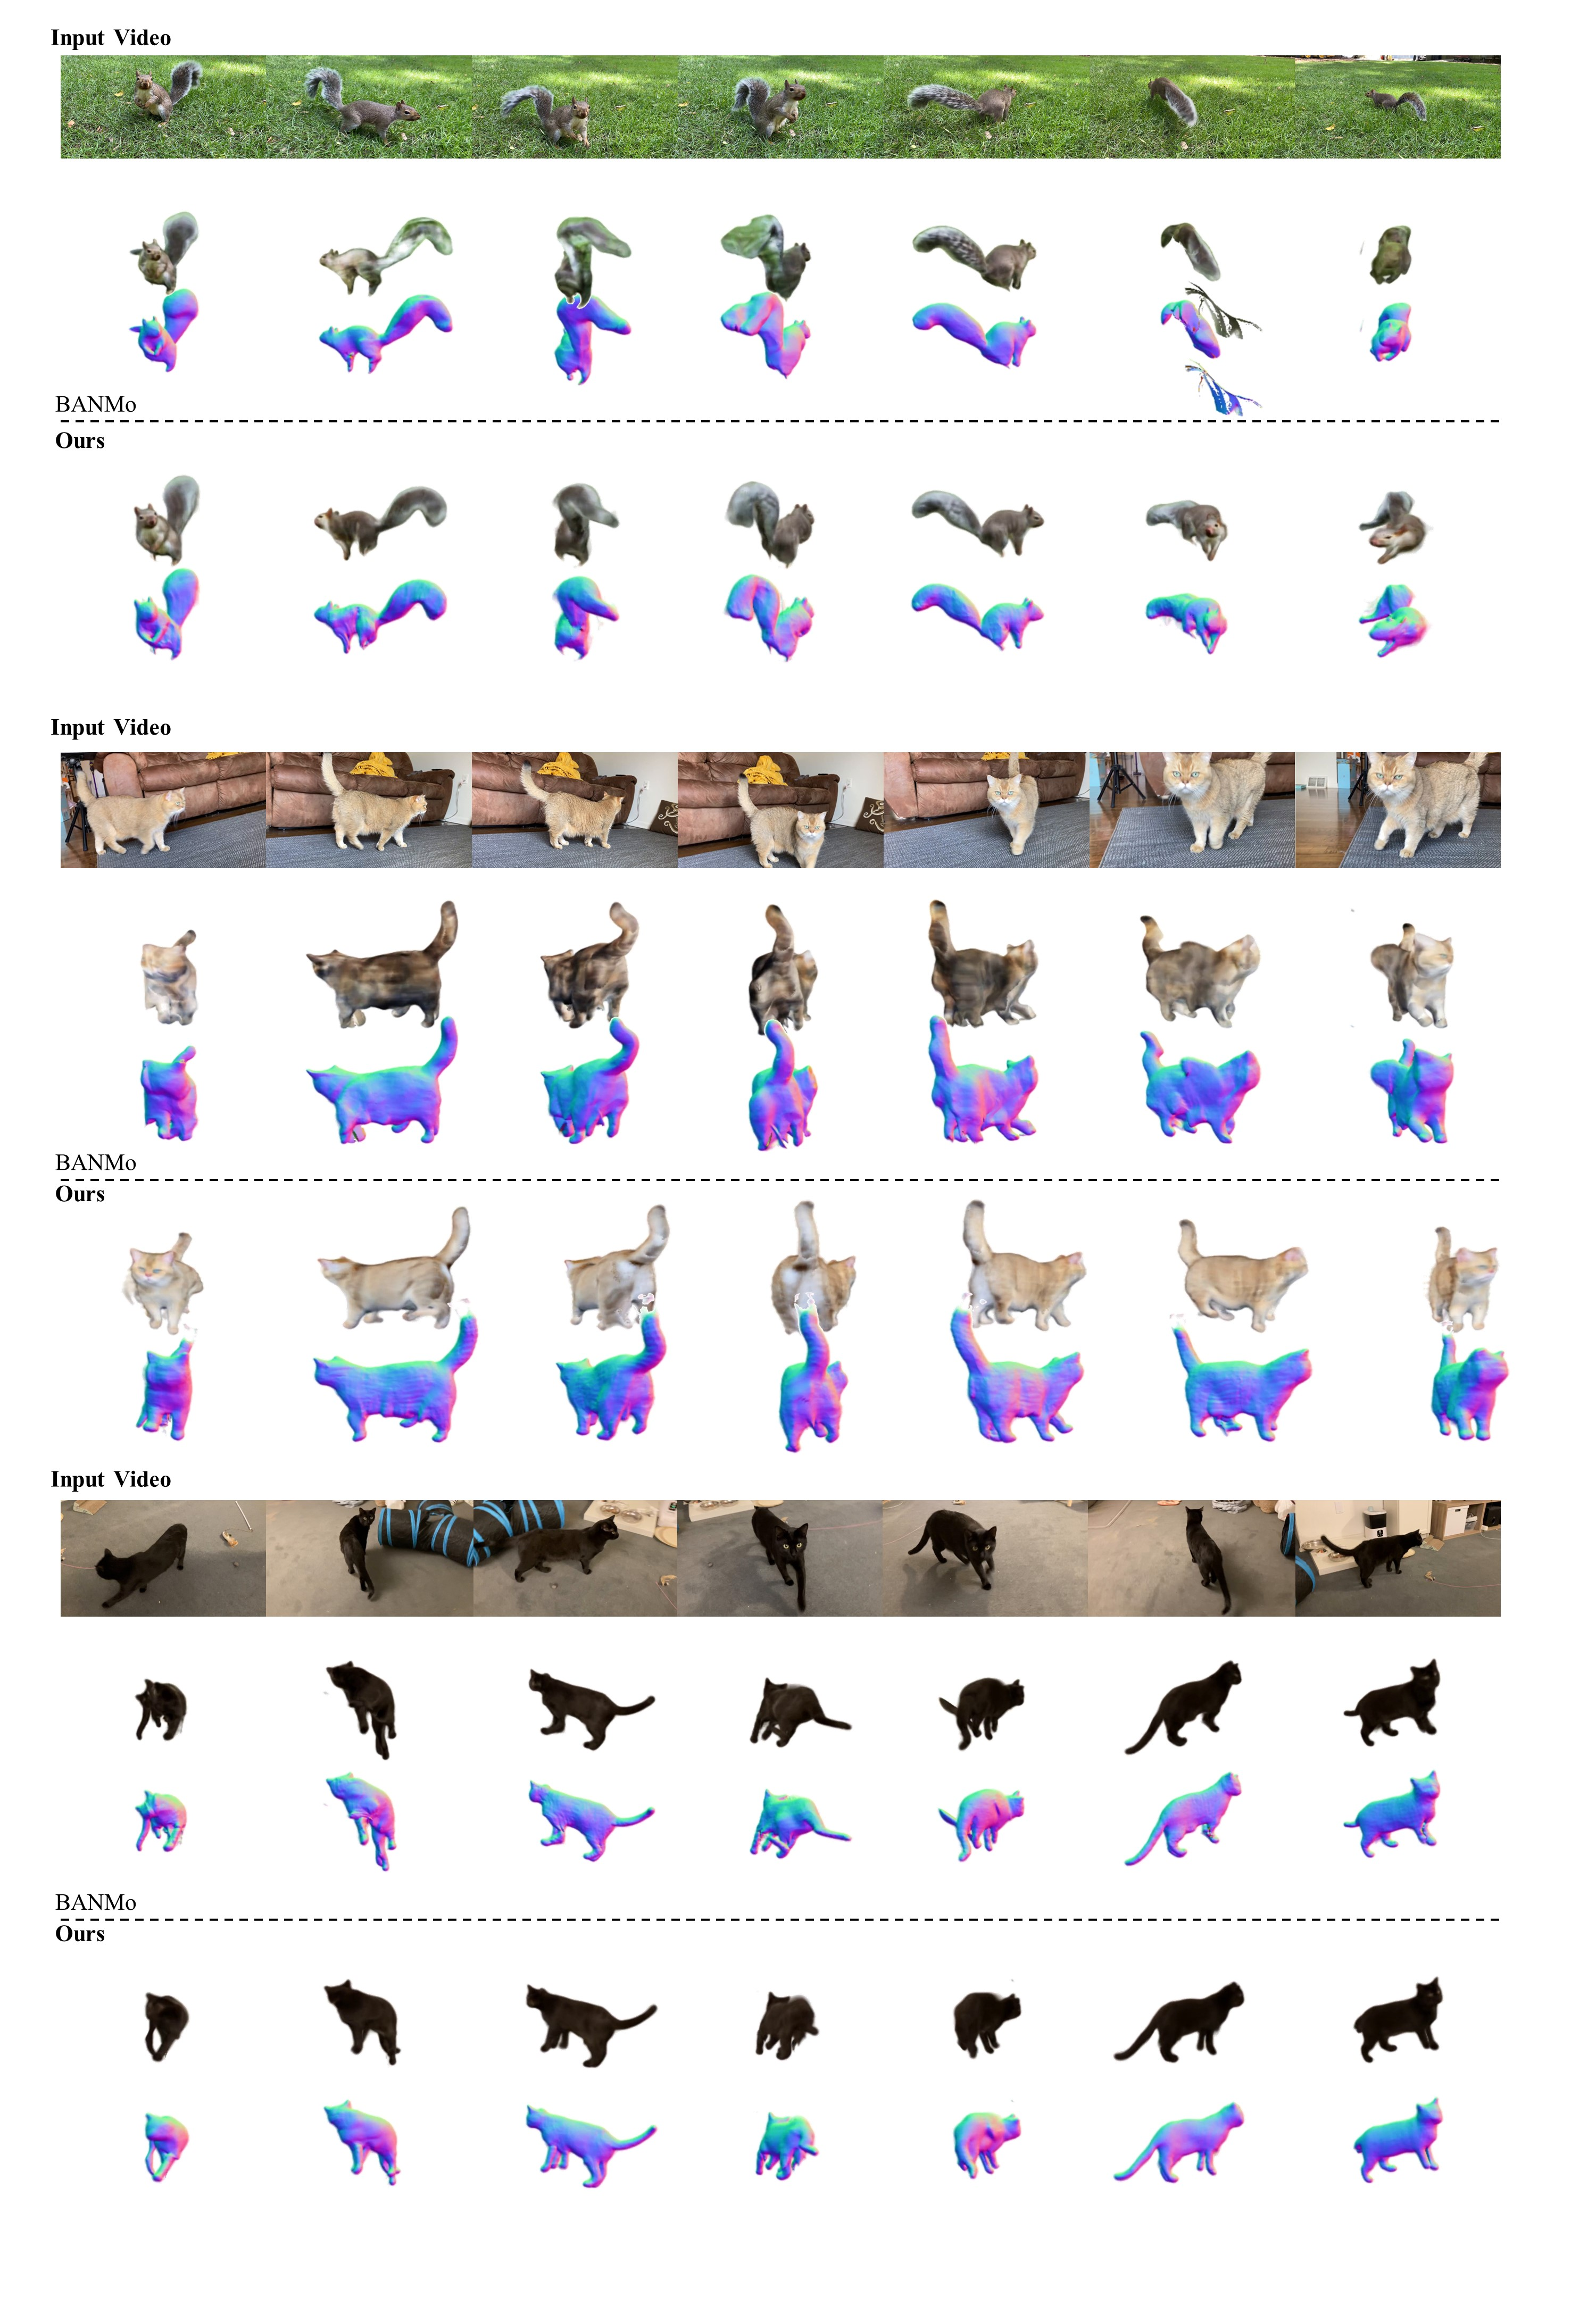}
   \caption{\textbf{More reconstruction result.} Our approach enhances the fidelity of the reconstructed models, particularly in regions not previously observed.}
   \label{fig:sup_recon}
\end{figure*}

\begin{figure*}[!h]
  \centering
  % \fbox{\rule{0pt}{2in} \rule{0.9\linewidth}{0pt}}
   \includegraphics[width=0.9 \linewidth]{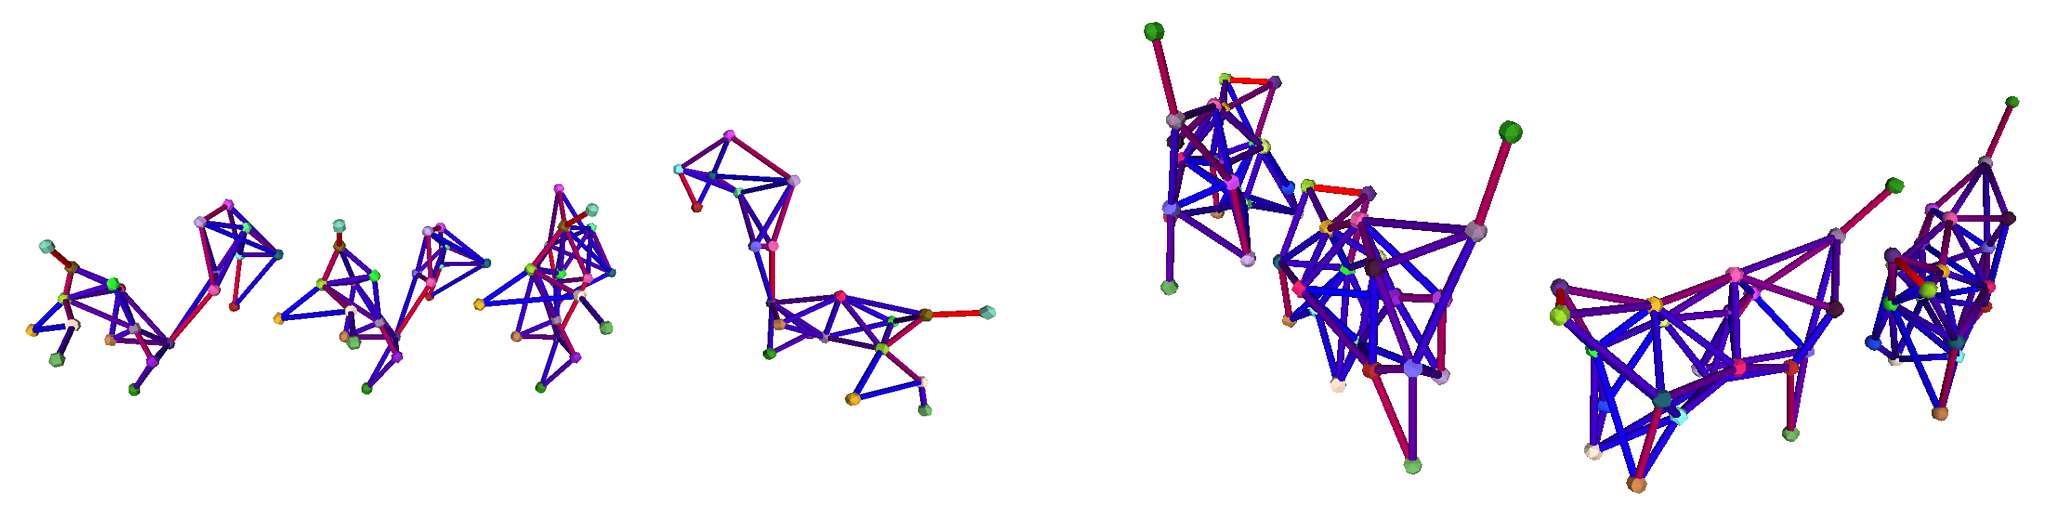}

   \caption{\textbf{The extracted skeletons with animations.} We extract skeletons associated with extended animations.}
   \label{fig:sup_anim}
\end{figure*}

% \section{Discussions of SDS and CSD}
% \begin{equation}
% \frac{\partial c_t}{\partial \phi}=\frac{\partial \mathcal{R}_{\phi_*}(\mathcal{W}_{\phi_w}^{t, \leftarrow}(\mathbf{X}^t))}{\partial \mathcal{W}_{\phi_w}^{t, \leftarrow}(\mathbf{X}^t)}   \frac{\partial \mathcal{W}_{\phi_w}^{t, \leftarrow}(\mathbf{X}^t)}{\partial \phi}
%     \label{eq:gradient}
% \end{equation}
% As $\mathcal{W}_{\phi_w}^{t, \leftarrow}(\mathbf{X}^t)$ are sampling points warped to canonical space via param, we replace it with $X^*$ for better understanding. It states that $\mathcal{W}_{\phi_w}^{t, \leftarrow}(\mathbf{X}^t)$ is independent of $\phi_*$, for it only warps the sample point from camera space to canonical space. So we have:
% \begin{equation}
% \frac{\partial c_t}{\partial \phi}=\frac{\partial \mathcal{R}_{\phi_*}(\mathbf{X}_*)}{\partial \mathbf{X}_*} \frac{\partial W_{\phi_w}^{t, \leftarrow}(\mathbf{X}_t)}{\partial \phi_w}
%     \label{eq:gradient2}
% \end{equation}

\section{Pseudo-code for AnimatableDreamer}
A more detailed pseudo-code for \textsc{AnimatableDreamer} is presented in \Cref{alg:CSD}.
\begin{algorithm}[!ht]
    \begin{algorithmic}[1]
        \Require{$\{I\}$, $\{t\}$, $\{\mathbf{p}\}$, $\mathbf{y}$}
        \Ensure{$\phi_{Gen}$}
        \State Initialize $\phi_{Recon}$
        \For{each $i \in [1,N]$} 

            \State Set position embedding bandwidth
            \If {i mod 2 == 0}
                \State $I,t,\mathbf{p}\leftarrow$ Sampler($\{I\}$, $\{t\}$, $\mathbf{p}$)
                \State $I_r\leftarrow$ Render($\phi_{Recon}$, $t$, $\mathbf{p}$)
                \State $\mathcal{L}\leftarrow(\mathcal{L}_{\text{Recon}}(I_r;I)+\mathcal{L}_{\text{Reg}})$
                \State Optimize $\phi_{Recon}$
            \Else
                \State $t,\mathbf{p}, T\leftarrow$ Sampler($\{t\}$, random pose, schedule)
                \State $I_r\leftarrow$ Render($\phi$, $t$, $\mathbf{p}$)
                \State $\mathcal{L}\leftarrow(\mathcal{L}_{\text{CSD}}(I_r;t,T,\mathbf{p},\mathbf{y})+\mathcal{L}_{\text{Reg}})$
                \State Freeze CameraMLP, Embedder
                \State Optimize $\phi_{Recon}$
                \State Unfreeze CameraMLP, Embedder
            \EndIf
        \EndFor
        \State Generate Skeletons $S$
        \State Initialize $\phi_{Gen}$ with $S$
        \For{each $i \in [1,N]$} 
            \State Set position embedding bandwidth
            \State Freeze CameraMLP, Embedder
            \State $t,\mathbf{p}, T\leftarrow$ Sampler($\{t\}$, random pose, schedule)
            \State $I_r\leftarrow$ Render($\phi$, $t$, $\mathbf{p}$)
            \State $\mathcal{L}\leftarrow(\mathcal{L}_{\text{CSD}}(I_r;t,T,\mathbf{p},\mathbf{y})+\mathcal{L}_{\text{Reg}}+\mathcal{L}_{\text{Skel}})$
            \State Optimize $\phi$
        \EndFor
    \State \Return {$\phi_{Gen}$}
    \end{algorithmic}
    \caption{Pseudo-code for AnimatableDreamer}
    \label{alg:CSD}
\end{algorithm}

This pseudo-code provides an overview of the CSD process, including initialization, sampling, rendering, loss calculation, and optimization steps for training the model. The Sampler function is responsible for extracting relevant information from input datasets, and the Render function renders images based on the current model parameters. The loss terms include reconstruction loss $\mathcal{L}_{\text{Recon}}$, CSD loss $\mathcal{L}_{\text{CSD}}$, and regularization loss $\mathcal{L}_{\text{Reg}}$.
Optimization of the reconstructed articulated model, denoted as $\theta_{Recon} $, is conducted in an alternating manner between the generation and the reconstruction loss functions. Subsequently, the extracted skeletons are utilized to steer the 4D generation process of $\theta_{Gen}$. It is noteworthy that both the CameraMLP and Embedder components are maintained in a frozen state when the optimization is driven by the generation loss $\mathcal{L}_{\text{Gen}}$.
\section{Weighting scalar $\alpha$ and threshold $\xi$}
In this study, the weighting scalar $\alpha$ and the threshold $\xi$ are determined through a hierarchical approach. The parameter $\alpha$ is optimized to ensure that geometrically distinct parts possessing similar semantic features are disconnected. Conversely, the threshold $\xi$ is established to facilitate the connection of skeletons with the top 80\% of scores. Subsequent to these adjustments, bones lacking a corresponding skeleton are eliminated.
\begin{figure}[!h]
\begin{minipage}[b]{0.5\textwidth}
  \begin{center}
      \includegraphics[width=0.9\linewidth]{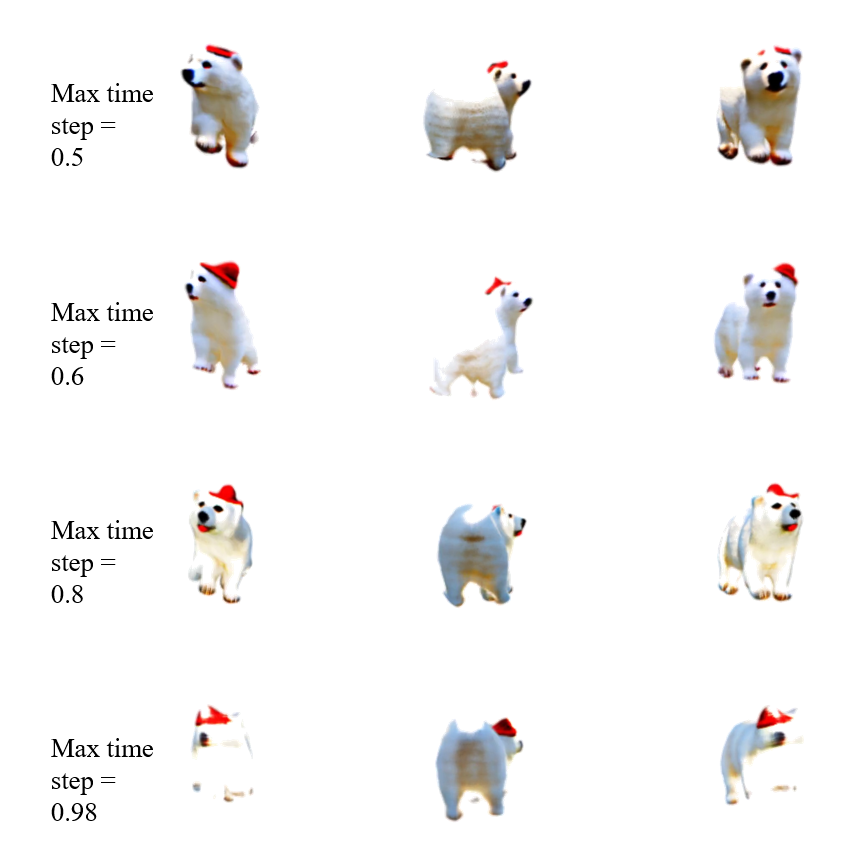}
      \vspace{-.5em}
      \caption{\textbf{The effect of the SDS time step.} The broader the range of the time step, the more significant the modifications to the model will be. An excessively large time step can compromise the integrity of the skeleton's structure, leading to erroneous results. Conversely, a time step that is too small may not induce sufficient changes in the model. Here we assign different time steps for reconstruction and generation.}
      \vspace{-1.5em}
      \label{fig:sdst}
  \end{center}
  \end{minipage}
  \hspace{0.5em}
  \begin{minipage}[b]{0.46\textwidth}
  \begin{center}
      \includegraphics[width=0.9\linewidth]{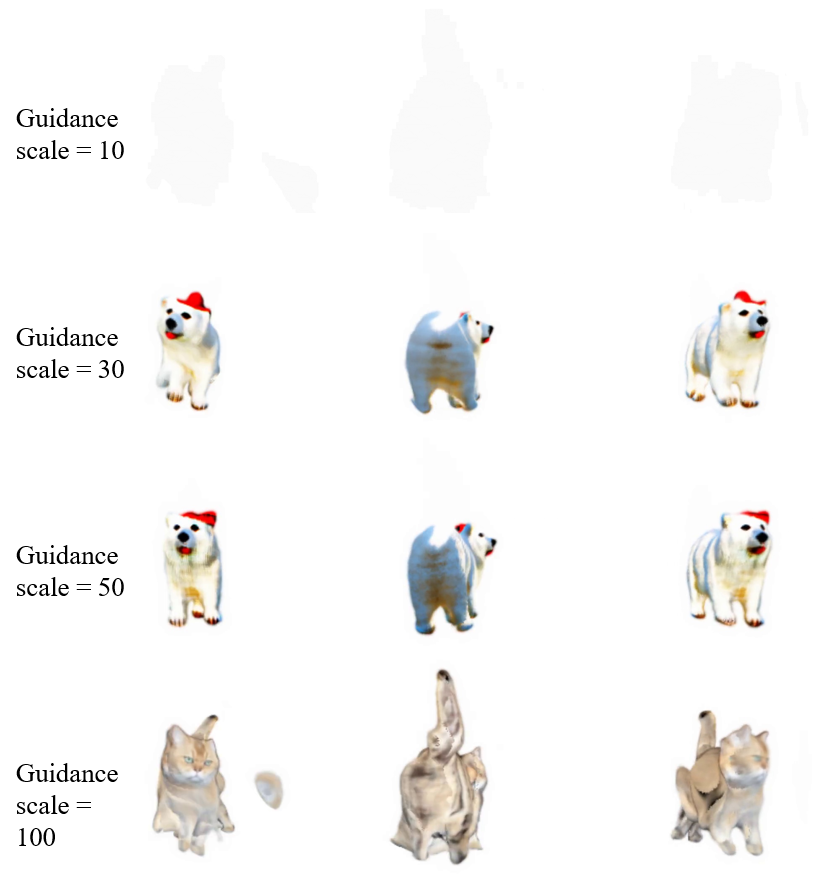}
      \vspace{-.5em}
       \caption{\textbf{Influence of guidance scale.} Setting CFG to 100 enhances the mode-seeking feature and almost bypasses the generation loss, while setting CFG to 10 results in the collapse of the 3D model. This behavior may be attributed to the strong constraints imposed by the articulation extracted from the template video, rendering high CFG unnecessary for ensuring the consistency of the diffusion model.}
      \vspace{-1.5em}
      \label{fig:gs}
  \end{center}
  \end{minipage}
\end{figure}

\section{Additional Details} 
\textbf{Hyper-parameters.} During the generation stage, the weight of $\mathcal{L}_{CSD}$ is progressively increased from 0 to 0.0001, while the weight of $\mathcal{L}_{reg}$ is adjusted according to a logarithmic function, ranging from 0.01 to 1. Throughout the skeleton extraction stage, the weight assigned to $\mathcal{L}_{CSD}$ is methodically reduced from 0.001 to 0.00001. Furthermore, given the disparate magnitudes of $\mathcal{L}_{skel}$ and $\mathcal{L}_{bone}$ in comparison to other loss terms, a balancing factor related to the dimensions of the canonical mesh is employed to maintain equilibrium. An AdamW optimization algorithm is utilized, configured with a learning rate of $5 \times 10^{-4}$.

\textbf{CSD is more CFG friendly.} 
For multi-view diffusion, the classifier-free guidance (CFG) weight is set to 50. In our experiments, we observe that setting CFG to around 30 yields the most beneficial results, as illustrated in \Cref{fig:gs}. This observation is attributed to the fact that the reconstruction loss aids in controlling the consistency of the generated content. However, for the reconstruction task, we have observed that setting CFG to a relatively large value is beneficial, as shown in Table 1. Therefore, we set CFG to 100 for the reconstruction process.

% \begin{table}[h]
%     \centering
%     \footnotesize
%     \setlength\tabcolsep{12pt}
%     \label{tab:abl_gs}
%     \begin{tabular}{c|c|c} %@{}
%       \toprule
%       Guidance scale  & CD  & F@$\%2$ \\
%       \midrule
%       10  &5.52& 44.8 \\
%       30  &5.33& 43.7 \\
%       50  &5.45& 45.5 \\
%       100  &4.6& 52.1\\
%       \bottomrule
%     \end{tabular}
%     \caption{\textbf{Ablation of the guidance scale in reconstruction.} A large guidance scale can ensure the consistency of the reconstructed model.}
% \end{table}

% \textbf{Diversity.} We also find that our method does not yield large amounts of diversity across random seeds. This may due to that SDS performs mode-seeking and $L_{recon}$ make it more mode-seeking for introducing a fixed geometry constrain. 
\textbf{CDS time step schedule.}
Given that our framework is a combination of both a generator and a reconstructor, we have carefully designed the SDS time step schedule based on a series of experiments. For prompts that induce significant changes in the object's geometry, we implement an annealing time step schedule ranging from 0.8 to 0.5. In cases where the prompt primarily affects texture or involves minimal geometry changes, we sample the time step in the range of 0 to 0.5. The impact of the SDS time step for generation is illustrated in \Cref{fig:sdst}. For reconstruction, we fix the time step to 0.5 after experiments (Table 2).

\begin{figure}[!h]
\centering
\begin{minipage}{.45\textwidth}
  \centering
  \footnotesize
  \setlength\tabcolsep{12pt}
  \begin{tabular}{c|c|c}
    \toprule
    Guidance scale & CD & F@\%2 \\
    \midrule
    10 & 5.52 & 44.8 \\
    30 & 5.33 & 43.7 \\
    50 & 5.45 & 45.5 \\
    100 & 4.6 & 52.1 \\
    \bottomrule
  \end{tabular}
  \captionof{table}{\textbf{Ablation of the guidance scale in reconstruction.} A large guidance scale can ensure the consistency of the reconstructed model.}
  \label{tab:abl_gs}
\end{minipage}%
\hfill
\begin{minipage}{.45\textwidth}
  \centering
  \footnotesize
  \setlength\tabcolsep{12pt}
  \begin{tabular}{c|c|c}
    \toprule
    Maximum $T$ & CD & F@\%2 \\
    \midrule
    0.5 & 4.6 & 52.1 \\
    0.8 & 5.06 & 47.8 \\
    0.98 & 4.68 & 49.1 \\
    \bottomrule
  \end{tabular}
  \captionof{table}{\textbf{Ablation of the time step schedule in reconstruction.} Setting the maximum \(T\) to an excessively large value can alter the original content and reduce the accuracy of reconstruction }
  \label{tab:abl_t}
\end{minipage}
\end{figure}

% \begin{table}[h]
%     \centering
%     \footnotesize
%     \setlength\tabcolsep{12pt}
%     \label{tab:abl_t}
%     \begin{tabular}{c|c|c} %@{}
%       \toprule
%       Maximum $T$ & CD  & F@$\%2$ \\
%       \midrule
%       0.5  &4.6& 52.1 \\
%       0.8 &5.06& 47.8 \\
%       0.98  &4.68& 49.1 \\
%       \bottomrule
%     \end{tabular}
%     \caption{\textbf{Ablation of the time step schedule in reconstruction.}}
% \end{table}
% \begin{figure}[ht]
%   \centering
%   % \fbox{\rule{0pt}{2in} \rule{0.9\linewidth}{0pt}}
%    \includegraphics[width=0.5\linewidth]{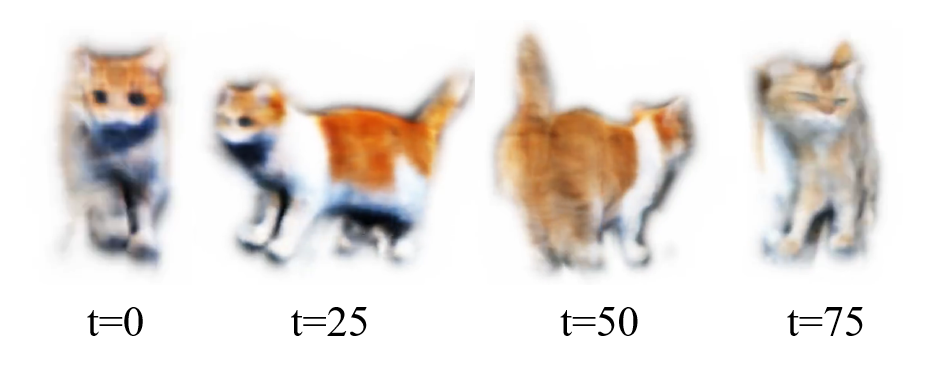}
%    \caption{\textbf{Time-invariant RGB ablation.} If we set the RGB values to be time-variant, we won't be able to cover all the points in the 4D space and consequently, the texture won't be time-consistent. For instance, the cat's face might look entirely different between the first frame and the last frame.}
%    \label{fig:abl_timefree}
% \end{figure}

\textbf{Near-far planes.} Given that we render from a free viewpoint rather than fixing on the reference, it is essential to compute the near-far plane of each frame dynamically. Therefore, our near-far planes are calculated on the fly to encompass all points of the proxy geometry with a considerable margin.

\textbf{Issue about MVDream.} MVDream is trained in a controlled environment where the object always faces the ``forward'' direction and is maintained at a proper distance from the camera. In contrast, our framework defines the ``forward'' direction based on the input video. To align the canonical model with the ``forward'' direction, we introduce an azimuth offset.

\textbf{The prompt impact result.} Our findings indicate that the incorporation of certain fixed negative prompts significantly benefits our task. Examples of these prompts include \textit{ugly, bad anatomy, blurry, pixelated}, and \textit{obscure}. Additionally, the inclusion of descriptors pertaining to the background proves advantageous, particularly in scenarios where the model's color closely resembles that of the background, thereby mitigating the risk of model disappearance.

\textbf{Time-invariant RGB.} 
Given the generally time-invariant appearance of the template object, we configure RGB as time-invariant to enhance the model's temporal consistency, especially when employing the CSD loss for reconstruction assistance.
% \subsubsection{Licenses}
% Here we provide the URL, citations and licenses of the open-sourced assets we use in this work.
% \subsection{User Study}

% ---- Bibliography ----
%
% BibTeX users should specify bibliography style 'splncs04'.
% References will then be sorted and formatted in the correct style.
%
% \bibliographystyle{splncs04}
% \bibliography{main}
